# Supplementary material for: Zero-shot Multi-level Feature Transmission Policy Powered by Semantic Knowledge Base
Source: arXiv:2305.12619 source file (2023-05-22)
Supplement: Supplementary file 1 [file appendix.tex]

\subsection{Proof of Lemma~\ref{lem:optB}}\label{app:optB}
Introduce $\mv C = \mv H \mv A \mv A^T \mv H^T + \sigma^2\mv I_K$ and $\tilde{\mv B} = \mv B \mv C^{\frac{1}{2}}$. By substituting $\mv B$ with $\tilde{\mv B} \mv C^{-\frac{1}{2}}$, problem~(P3) is reformulated as 
\begin{align}
    \text{(P10)}\  & \min_{\tilde{\mv B}}\ \  -\text{Tr}\left(\mv U_R\mv \Lambda_R^{-1}\tilde{\mv B}  \mv C^{-\frac{1}{2}}\mv H\mv A\right)\nonumber \\
    &\  s.t. \ \ \  \text{Tr}\left(\tilde{\mv B}\tilde{\mv B}^T\right) \leq 1. \label{eq:consBB2}
\end{align}

Let $\mu \geq 0$ be the dual variable associated with constraint (\ref{eq:consBB2}). The partial Lagrangian of problem~(P3) can be expressed as 
\begin{align}
   & \mathcal{L}(\tilde{\mv B},\mu) %\nonumber\\
  % & =  -\mathbb{E}\left( \hat{\mv s}^T \left(\mv B\mv H\mv A\mv d + \mv B\mv n\right)\right) + \mu \left(\mathbb{E}\left(\|\mv B\mv H\mv A\mv d + \mv B\mv n\|^2\right) \right) \nonumber\\
   %& - \mu \nonumber\\
    = -\text{Tr}\left(\mv U_R\mv \Lambda_R^{-1}\tilde{\mv B}  \mv C^{-\frac{1}{2}} \mv H\mv A\right)   + \mu \text{Tr}\left(\tilde{\mv B}\tilde{\mv B}^T\right) - \mu.\nonumber
   % & - \mu. 
\end{align}
The derivative of $\mathcal{L}(\tilde{\mv B},\mu)$ w.r.t. matrix $\tilde{\mv B}$ is given as
\begin{align}
    \frac{\partial \mathcal{L}(\tilde{\mv B},\mu)}{\partial \tilde{\mv B}} = -\mv C^{-\frac{1}{2}}\mv H \mv A \mv U_R \mv \Lambda_R^{-1} + 2\mu \tilde{\mv B}^T. \nonumber%\label{eq:partialB}\nonumber
\end{align}

Accordingly, the KKT conditions are given as
\begin{align}
   &-\mv C^{-\frac{1}{2}}\mv H \mv A \mv U_R \mv \Lambda_R^{-1} + 2\mu \tilde{\mv B}^T =  0,\label{eq:first0}\\
   & \mu\left( \text{Tr}\left(\tilde{\mv B}\tilde{\mv B}^T\right) - 1\right) = 0,\label{eq:kkt1}\\
   & \mu \geq 0,\label{eq:kkt2}\\
   & \text{Tr}\left(\tilde{\mv B}\tilde{\mv B}^T\right)\leq 1. \label{eq:kkt3}
\end{align}

From (\ref{eq:first0}) and (\ref{eq:kkt2}), we have when $\mu = 0$, the equation in (\ref{eq:first0}) does not hold. Thus, $\mu > 0$, and 
\begin{align}
   \tilde{\mv B}^T = \frac{1}{2\mu} \mv C^{-\frac{1}{2}}\mv H \mv A \mv U_R \mv \Lambda_R^{-1}. \label{eq:optBt}
\end{align}

Then, since $\mu>0$, from (\ref{eq:kkt1}) we have 
\begin{equation}
 \text{Tr}\left(\tilde{\mv B}\tilde{\mv B}^T\right) = 1. \label{eq:eq1}
\end{equation}

Via substituting (\ref{eq:optBt}) into (\ref{eq:eq1}), we have 
%By setting $\frac{\partial \mathcal{L}(\mv B,\mu)}{\partial \mv B} = 0$, we have 
%By letting $\mathbb{E}\left(\|\mv B\mv H\mv A\mv d + \mv B\mv n\|^2\right) = 1$, we have
\begin{align}
   & \mu =\frac{1}{2}\sqrt{\text{Tr}\left(\mv \Lambda_R^{-2}\mv U_R^T\mv A^T\mv H^T\mv C^{-1} \mv H \mv A \mv U_R\right)}. 
\end{align}
The proof ends.

%By substituting (\ref{eq:optAt}) into (\ref{eq:eq2}), we have
%\begin{align}
%    \mu_2 = 
%\end{align}

%If $\mu_1=0$ and $\mu_2 = 0$ hold simultaneously, $\frac{\partial \mathcal{L}(\mv A,\mu_1,\mu_2)}{\partial \mv A} = -\mv U_0\mv \Lambda_0^{-1}\mv B \mv H$, which is independent of $\mv A$. Thus, $f(\mu_1,\mu_2)$ is unbounded. The proof ends. 

%\subsection{Proof of  Lemma~\ref{lem:optA}} \label{app:optA2}
%By setting $\frac{\partial \mathcal{L}(\mv A,\mu_1,\mu_2)}{\partial \mv A} = 0$, we have 
%\begin{align}
%    \mv A^T = \frac{1}{2}\mv U_0\mv \Lambda_0^{-1}\mv B \mv H  \left(\mu_1 \mv I_K + \mu_2\mv H \mv B^T\mv B\mv H\right)^{-1}. 
%\end{align}
%The proof ends. 

%Via substituting $a_i$ in (\ref{eq:optai2}) into $\sum_{i=1}^k a_i  = \bar{E}$, we have
%\begin{align}
%    \frac{1}{\sqrt{2\beta \alpha}} = \frac{\bar{E}+\sum_{i=1}^k \frac{\sigma^2}{h_i^2}}{\sum_{i=1}^k\frac{\sigma}{h_i\lambda_i}}. \label{eq:optalpha}
%\end{align}
%Via substituting (\ref{eq:optalpha}) into (\ref{eq:optai1}), (\ref{eq:optai}) holds. 

\subsection{Proof of Theorem~\ref{the:pergua}}\label{app:pergua}
Via substituting $\mv A$ with $\mv A^*$ and $\mv B$ with $\mv B_{\text{opt}}(\mv A^*)$, the cosine similarity in (\ref{eq:expcosim}) is given as (\ref{eq:pergua}).
%\begin{align}
%    \text{cosim}(\mv A^*,\mv B_{\text{opt}}(\mv A^*)) = \sqrt{1 - \frac{\left(\sum_{i=1}^k \frac{\sigma}{\lambda_ih_i}\right)^2}{\left(\bar{E} + \sum_{i=1}^k \frac{\sigma^2}{h_i^2}\right)\sum_{i=1}^k \lambda_i^{-2}}}. 
%\end{align}
Since the optimal cosine similarity $\text{cosim}^*$ is no larger than $1$, we have
\begin{align}
    \frac{\text{cosim}(\mv A^*,\mv B_{\text{opt}}(\mv A^*))}{\text{cosim}^*}  \geq \text{cosim}(\mv A^*,\mv B_{\text{opt}}(\mv A^*)). 
\end{align}
The proof ends.
